# Supplementary material for: Deep PatchMatch MVS with Learned Patch Coplanarity, Geometric Consistency and Adaptive Pixel Sampling
Source: arXiv:2210.07582 source file (2022-10-14)
Supplement: Supplementary file 3 [file supp.tex]

%\input{tex/supp/ablation_on_high_resolution}
%\input{tables/supp/ablation_hr}
%\input{tables/supp/ablation_additional}
%\input{tex/supp/additional_ablations}
%\input{tex/supp/additional_vis}
%\input{figures/supp/eth3d_hr_train}
%\input{figures/supp/eth3d_hr_test}
%\input{figures/supp/eth3d_lr_train}
%\input{figures/supp/eth3d_lr_test}
%\input{figures/supp/tnt}
%\input{figures/supp/tnt_advanced}
