# Supplementary material for: Deep PatchMatch MVS with Learned Patch Coplanarity, Geometric Consistency and Adaptive Pixel Sampling
Source: arXiv:2210.07582 source file (2022-10-14)
Supplement: Supplementary file 5 [file ablation_on_high_resolution.tex]

\section{Ablations on High-Resolution Images}
Table~\ref{tab:ablation_hr} shows additional ablation studies on $\text{Ours}_{hr}$ which uses 10 images of resolution of $3200 \times 2112$ for each view. We show that the ablation on $\text{Ours}_{hr}$ shows similar results to $\text{Ours}_{lr}$. 
Having Geometric consistency improves the $F_1$ score by 1.6\% at the 2cm threshold, and 1.2\% at the 5cm threshold.
Without Geometric consistency, the $F_1$ score drops by 0.7\% at the 2cm threshold and 0.5\% at the 5cm threshold.
U-Net~\cite{ronneberger2015u} based feature extractor improves the $F_1$ score by 2.3\% and 1.8\% at the 2cm and the 5cm threshold. Without U-Net~\cite{ronneberger2015u} based feature extractor, the $F_1$ score drops by 1.4\% at the 2cm threshold and 1.3\% at the 5cm threshold.
Learned coplanarity improves the overall $F_1$ score by 1.4\% at the 2cm threshold and 1.0\% at the 5cm threshold.
Without the learned coplanarity, the $F_1$ score drops by 1.0\% at both thresholds.
